# Supplementary material for: Variational Hamiltonian simulation for translational invariant systems via classical pre-processing
Source: arXiv:2106.03680 source file (2023-03-06)
Supplement: Supplementary file 1 [file appendixB.tex]

Given a translational invariant $k$-nearest neighbor Hamiltonian $H$ on $N$ qubits, we can describe it by two indices, $a \in \{1, ..., A\}$ which labels the types of interactions and $n \in \{1, ..., N\}$ which labels the first qubit on which the interaction term $H_{n, a}$ acts. Altogether,
\begin{align}
    H = \sum_{n, a} c_{a} H_{n, a}.
\end{align}
For instance, the \model model is described by $H_{n, 1} = Z_n Z_{n+1}, c_{1}=J_z$ and $H_{n, 2} = X_n, c_{2}=h_x$, modulo periodic boundary conditions. In the following, we will need to specify an ordering of the terms to not confuse non-commuting terms. We will choose to order two pairs of indices $(n, a) \leq (n', a')$, if $n<n'$ or if $n = n'$ and $a \leq a'$. We will write $(n, a)< (n', a')$, if $(n, a) \leq (n', a')$ and $(n, a) \neq (n', a')$ holds. Of course, this choice of ordering is not unique but rather a matter of choice.

The time evolution generated by $H$ can then be approximated by a first order product formula
\begin{align}
    \Uex = e^{-it H} = \left( \prod_{n, a}^\leftarrow e^{-i\frac{t}{m} c_{a} H_{n, a}} \right)^m - \mathcal{A}_T
    \label{eq:Trot_error}
\end{align}
where the arrow $\leftarrow$ denotes an operator ordering beginning with $(1, 1)$ and $\mathcal{A}_T$ is the additive Trotter-Error, given by the leading order
\begin{align}
    \mathcal{A}_T = \frac{t^2}{2m} \sum_{(n, a) < (n', a')} c_{a} c_{a'} \left[ H_{n', a'}, H_{n, a} \right] + \mathcal{O}(t^3)
\end{align}
for the first order Trotter-Suzuki decomposition. If we instead decide to use a variational gate sequence to approximate time evolution, we need to modify (\ref{eq:Trot_error}) in the following way
\begin{align}
    \Uex = \left( \prod_{n, a}^\leftarrow e^{-i\frac{t}{m} c_{a} H_{n, a}} \right)^m \left( \prod_{n, a}^\rightarrow e^{i\frac{t}{m} c_{a} H_{n, a}} \right)^m \left( \prod_{r=1}^m \prod_{n, a}^\leftarrow e^{-i \theta_{r, a} H_{n, a}} \right) - \mathcal{A}_T - \mathcal{A}_V
    \label{eq:Var_error}
\end{align}
where $\theta_{r, a}$ denotes the variational parameter which is dependent on the layer number $r$ and the interaction type $a$ but not on the qubit $n$. In order to correct for the changes made, the additive error $\mathcal{A}_V$ has been added. Up to cubic order in $t$ or $\theta$, respectively, it reads
\begin{align}
    \mathcal{A}_V = \Uex \left[ \left( \prod_{n, a}^\rightarrow e^{i\frac{t}{m} c_{a} H_{n, a}} \right)^m \left( \prod_{r=1}^m \prod_{n, a}^\leftarrow e^{-i \theta_{r, a} H_{n, a}} \right) - \mathds{1} \right] + \mathcal{O} (t^3),
    \label{eq:AV}
\end{align}
which can be verified by plugging in (\ref{eq:AV}) into (\ref{eq:Var_error}). Here and in the following, we omit other cubic order terms of the form $t^2 \theta, \theta^2 t, \theta^3$ and write $t^3$ only as we assume the parameters $\theta$ to be of order $t$. Since $\Uex$ has a $0^\text{th}$ order and the rest of the operator has only contributions linear in $t$, the newly introduced error $\mathcal{A}_V$ will be linear in $t$. Although, this worsens the asymptotic behavior in $t \to 0$, we can achieve an optimization for a fixed single step time $t$. Gathering all the linear and quadratic terms in $t$ and/or $\theta$, we find
\begin{align}
    \mathcal{A}_V + \mathcal{A}_T = i t H + \frac{t^2}{2} H^2 
    - \Bigg[ 
    &i\sum_{a} \left( \sum_{r} \theta_{r, a} \right) \left( \sum_n H_{n, a} \right)
    + \sum_{a, a'} \left( \sum_{r<r'} \theta_{r', a'} \theta_{r, a} \right) \left( \sum_{n, n'} H_{n, a} H_{n', a'} \right) \nonumber \\
    &+ \frac{1}{2} \sum_{a} \left( \sum_{r} \theta_{r, a}^2 \right) \left( \sum_n H_{n, a}^2 \right)
    + \sum_{(n', a')< (n, a)} \left( \sum_{r} \theta_{r, a} \theta_{r, a'} \right) H_{n', a'} H_{n, a}
    \Bigg].
    \label{eq:sum_error}
\end{align}
Note that all terms are no longer of $k$ nearest-neighbor type, in general, but rather can act on any $2k$ qubits in the system. These operators can be used to minimize $\mathcal{A}_V + \mathcal{A}_T$ on an $N$ qubit system. We can see the optimization potential better by rewriting the variational parameters into $\theta_{r, a} = \frac{t c_a}{m} + \Delta_{r, a}$:
\begin{align}
    \mathcal{A}_V + \mathcal{A}_T &= \frac{t^2}{2m} \sum_{(n, a) < (n', a')} c_{a} c_{a'} \left[ H_{n', a'}, H_{n, a} \right] \nonumber \\
    &- \Bigg[ 
    i\sum_{a} \left( \sum_{r} \Delta_{r, a} \right) \left( \sum_n H_{n, a} \right) \nonumber \\
    &+ \frac{t}{m} \sum_{a, a'} \left( \sum_{r} ((r-1) c_a \Delta_{r, a'} + (m-r) c_{a'} \Delta_{r, a}) + \sum_{r<r'} \Delta_{r', a'} \Delta_{r, a} \right) \left( \sum_{n, n'} H_{n, a} H_{n', a'} \right) \nonumber \\
    &+ \sum_{a} \left( \sum_{r} \left( \Delta_{r, a} \frac{t}{m} c_a + \frac{\Delta_{r, a}^2}{2} \right) \right) \left( \sum_n H_{n, a}^2 \right) \nonumber \\
    &+ \sum_{(n', a')< (n, a)} \left( \sum_{r} \left( (\Delta_{r, a} c_{a'} + \Delta_{r, a'} c_a) \frac{t}{m} + \Delta_{r, a} \Delta_{r, a'} \right) \right) H_{n', a'} H_{n, a}
    \Bigg].
    \label{eq:Var_error_Delta}
\end{align}
The first term resembles the first order Trotter error (\ref{eq:Trot_error}). The rest is at least linear in $\Delta$. Hence, the choice $\Delta_{r, a} = 0 \, \forall r, a$ corresponds to the parameters of the Trotter-Suzuki decomposition. A non-trivial set of $\Delta_{r, a}$ on the other hand could use the operators in (\ref{eq:Var_error_Delta}) to correct on the commutator terms of the leading order Trotter error. To completely decouple the optimal parameters $\Delta$ from the qubit index $n$ in (\ref{eq:Var_error_Delta}), we rewrite the sums
\begin{align}
    \sum_{(n', a') < (n, a)} H_{n', a'} H_{n, a} = \frac{1}{2} \sum_{(n', a') \neq (n, a)} H_{n', a'} H_{n, a} + \frac{1}{2} \sum_{(n', a') < (n, a)} [H_{n', a'}, H_{n, a}],
\end{align}
and use the $k$-locality of the Hamiltonian to get rid of vanishing commutators. We arrive at
\begin{align}
    \mathcal{A}_V + \mathcal{A}_T &= \frac{t^2}{2m} \sum_n \left( \sum_{a < a'} c_{a} c_{a'} \left[ H_{n, a'}, H_{n, a} \right] + \sum_{a', a} \sum_{l = 1}^{k-1} c_{a} c_{a'} \left[ H_{n+l, a'}, H_{n, a} \right] (2 \Theta(N-n-l) - 1) \right) \nonumber \\
    &- \Bigg[ 
    i\sum_{a} \left( \sum_{r} \Delta_{r, a} \right) \left( \sum_n H_{n, a} \right) \nonumber \\
    &+ \frac{t}{m} \sum_{a, a'} \left( \sum_{r} ((r-1) c_a \Delta_{r, a'} + (m-r) c_{a'} \Delta_{r, a}) + \sum_{r<r'} \Delta_{r', a'} \Delta_{r, a} \right) \left( \sum_{n, n'} H_{n, a} H_{n', a'} \right) \nonumber \\
    &+ \sum_{a} \left( \sum_{r} \left( \Delta_{r, a} \frac{t}{m} c_a + \frac{\Delta_{r, a}^2}{2} \right) \right) \left( \sum_n H_{n, a}^2 \right) \nonumber \\
    &+ \sum_{(n', a') \neq (n, a)} \left( \sum_{r} \left( (\Delta_{r, a} c_{a'} + \Delta_{r, a'} c_a) \frac{t}{m} + \Delta_{r, a} \Delta_{r, a'} \right) \right) H_{n', a'} H_{n, a} \nonumber \\
    &+ \sum_{n} 
    \left( \sum_{a'< a} \xi_{a, a'} \left[ H_{n, a'}, H_{n, a} \right] + \sum_{a', a} \xi_{a, a'} \sum_{l = 1}^{k-1} \left[ H_{n, a'}, H_{n+l, a} \right] (2 \Theta(N-n-l) - 1) \right) \Bigg],
    \label{eq:Var_error_Delta_final}
\end{align}
where $\xi_{a, a'} = \left( \sum_{r} \left( (\Delta_{r, a} c_{a'} + \Delta_{r, a'} c_a) \frac{t}{m} + \Delta_{r, a} \Delta_{r, a'} \right) \right)$ is a shorthand for the variational coefficient and $\Theta$ denotes the Heavyside step function and corrects relative signs which are due to the ordering inherited from the first order Trotter sequence which do not involve periodic boundary effects. Any commutator which acts accross the boundary gathers a minus sign in the first as well as in the last line. In the form of (\ref{eq:Var_error_Delta_final}), it is straight forward to extract those operators which only differ by the qubits, they are acting on.

Let us assume, we have performed an optimization to minimize $\mathcal{A}_V + \mathcal{A}_T$ such that
\begin{align}
    \frac{1}{2^N} || \mathcal{A}_V + \mathcal{A}_T ||_F^2 < \epsilon
\end{align}
with $\epsilon > 0$. As $\mathcal{A}_V + \mathcal{A}_T$ is still translationally invariant, we can understand the remaining error as a sum of equal contributions
\begin{align}
    \mathcal{A}_V + \mathcal{A}_T = \sum_{n} \frac{E_{n}}{N} \qquad \text{with } \quad ||E_{n}|| < 2^N \epsilon \quad \forall n
\end{align}
If we were to add one qubit to the system and fix the boundary conditions adequately, we need to delete terms which describe interactions along the former periodic boundary and add new terms. The new Hamiltonian will take the form
\begin{align}
    H \otimes \mathds{1} + \sum_a \sum_{l=0}^{k_a-1} \left( \tilde H_{N+1-l, a}\right)  - \sum_a \sum_{l=0}^{k_a-2} \left( H_{N-l, a} \otimes \mathds{1} \right)
\end{align}
where the qubit index $n$ is identified via $k \leftrightarrow N+k$ for the terms $H_{n, a}$ and modulo $k \leftrightarrow N+1+k$ for $\tilde H_{n, a}$. $k_a$ denotes the number of neighboring qubits on which the term $H_{n, a}$ (or $\tilde H_{n, a}$, respectively) acts. Hence, we effectively raise the sums in $n$ in (\ref{eq:sum_error}, \ref{eq:Var_error_Delta}) by $A$ many addends per sum. By the same argument as before the terms of equal error contributions rise in the following way

\begin{align}
    || \mathcal{A}_V^{(N)} + \mathcal{A}_T^{(N)} ||_F^2 \longrightarrow || \mathcal{A}_V^{(N+1)} + \mathcal{A}_T^{(N+1)} ||_F^2 < 2^{N+1} \frac{N+1}{N} \epsilon.
\end{align}
By iteration over the number of added qubits $K$ we get
\begin{align}
    || \mathcal{A}_V^{(N+K)} + \mathcal{A}_T^{(N+K)} ||_F^2 < 2^{N+K} \frac{N+K}{N} \epsilon.
\end{align}
