# Supplementary material for: Variational Hamiltonian simulation for translational invariant systems via classical pre-processing
Source: arXiv:2106.03680 source file (2023-03-06)
Supplement: Supplementary file 2 [file appendixC.tex]

\begin{figure}
    \centering
    \includegraphics{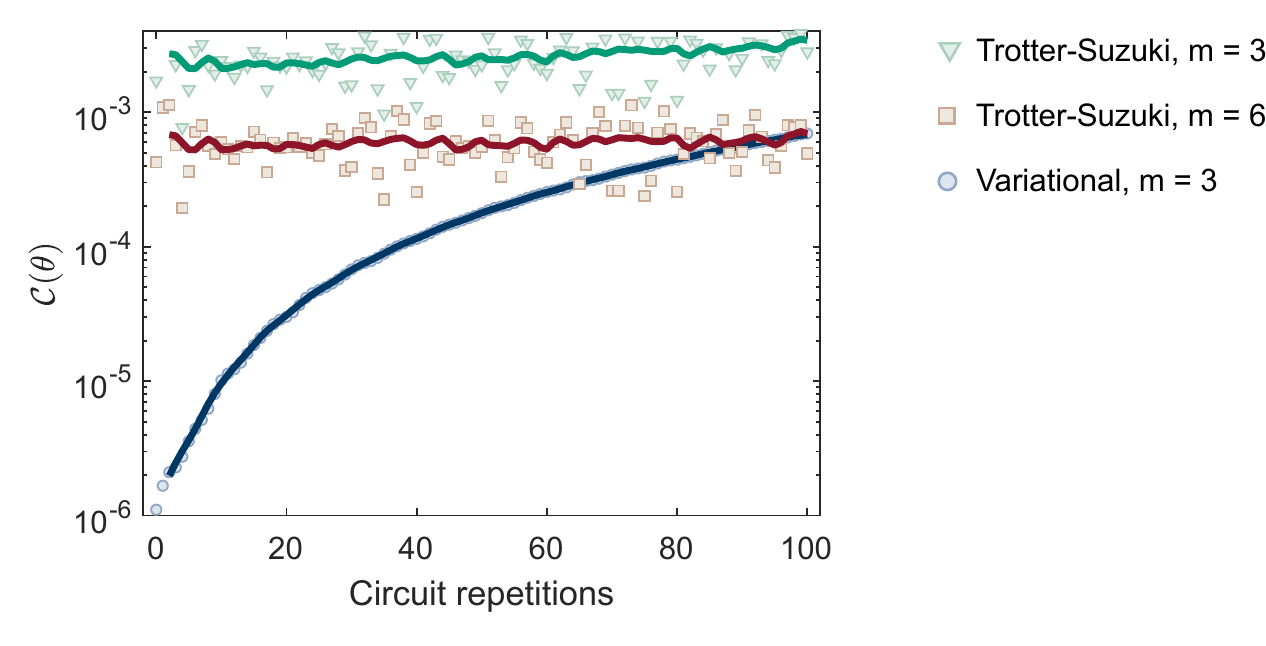}
    \caption{Trace Distance of variational vs. Trotter gate sequence from the exact output state of a simulation of up to 100 time steps. The interaction strengths of the \model model read $J_z=1.0, h_x = 0.25$. A single time step is $t = 0.3$ and the system geometry is a $3 \times 3$ square lattice.}
    \label{fig:tr_dist}
\end{figure}

In section \ref{sec:Opt}, we introduced the cost function (\ref{eq:Frob_cost}) which represents a measure of distance on unitaries induced by the Frobenius norm. The choice of cost function is actually not unique. One could, for instance, choose another norm to define
\begin{align}
    C(\theta) = \alpha ||U_\text{target} - U_\text{var}(\theta)||^2,
    \label{eq:mod_cost}
\end{align}
with $\alpha$ some constant and $||.||$ denoting an arbitrary matrix norm. The operator norm would be a natural choice, as it describes an upper bound to any element of $U_\text{target} - U_\text{var}(\theta)$. For an optimization routine, however, the cost function needs to be continuously differentiable, which is not given by the operator norm, in general.

A smooth candidate would be a Schatten $p$-norm defined by
\begin{align}
    ||U_\text{target} - U_\text{var}(\theta)||_p = \left[\Tr{ \left( |U_\text{target} - U_\text{var}(\theta) |^p \right) } \right]^\frac{1}{p}.
\end{align}
To avoid calculating the absolute of the operator $U_\text{target} - U_\text{var}(\theta)$, one is tempted to choose an even $p$, such as $p=2$ which already yields the Frobenius norm. In fact, any other norm yields a similar behavior. The trace norm ($p=1$) is of particular interest as it provides a tighter upper bound to the error on the expectation value of any observable
\begin{align}
    |\braket{\psi |\Uex^\dagger \mathcal{O} \Uex - \Uvar^\dagger \mathcal{O} \Uvar |\psi}| \leq 2 ||\mathcal{O}|| ||\Uex - \Uvar||_1
\end{align}
In Figure \ref{fig:tr_dist}, we plot a modified cost function (\ref{eq:mod_cost}) induced by the trace distance to the exact output state and compare variational vs. Trotter sequence. Not very surprisingly, the orders of magnitude and the overall trend behaves very similar to the cost function induced by the Frobenius distance.
